# Supplementary material for: High-dimensional multi-input quantum random access codes and mutually unbiased bases
Source: arXiv:2111.08890 source file (2022-10-15)
Supplement: Supplementary file 1 [file Supplemental_Material.pdf]

# Supplemental Material: High-Dimensional Multi-input Quantum Random Access Codes and Mutually Unbiased Bases

Rui-Heng Miao *[,1,2,3], Zhao-Di Liu †[,1,2,3], Yong-Nan Sun ‡[,4,1,2], Chen-Xi Ning[1,2,3], Chuan-Feng Li §[,1,2,3] and Guang-Can Guo[1,2,3]

[1] *CAS Key Laboratory of Quantum Information, University of Science and Technology of China, Hefei 230026, China*
[2] *CAS Center For Excellence in Quantum Information and Quantum Physics, University of Science and Technology of China, Hefei 230026, China*
[3] *Hefei National Laboratory, University of Science and Technology of China, Hefei 230088, China*
[4] *Department of Physics, Hangzhou Normal University, 311121 Hangzhou, Zhejiang, China*

## Contents

**1 Proof of $P_{3d}^{QM} > P_{3d}^{C}$** **1**

**2 List of $P_{3d}^{QM}$ in Operational Inequivalence of MUBs in $3^{(d)} \to 1$ QRACs** **2**

**3 Proving MUBs Are Not The Optimal Measurement Bases** **3**

**4 Visibility of Laguerre-Gaussian Mode When $d = 11$** **4**

**5 The Bases We Used in The Experiment of $3^{(d)} \to 1$ QRACs** **5**

**6 The Experimental Results of QRACs** **8**

## 1 Proof of $P_{3d}^{QM} > P_{3d}^{C}$

Here $P_{3d}^{C}$ represents the maximum success probability of the $3^{(d)} \longrightarrow 1$ random access codes (RACs). We have got the analytical solution of the maximum success probability of QRACs when measurement bases are MUBs,

$$P_{3d}^{QM} = \frac{1}{3d^3} \sum_{x_0=0}^{d-1} \sum_{x_1=0}^{d-1} \sum_{x_2=0}^{d-1} \left( 1 + \frac{2}{\sqrt{d}} \cos \frac{\Phi(x_0,\ x_1,\ x_2)}{3} \right). \tag{1}$$

Here $\Phi(x_0,\ x_1,\ x_2) \in [-\pi, \pi)$, $\cos \frac{\Phi(x_0,\ x_1,\ x_2)}{3} \geqslant \frac{1}{2}$, so the lower bound of $P_{3d}^{QM}$ is $\frac{1}{3}\left(1 + \frac{1}{\sqrt{d}}\right)$, and we have already know the maximum success probability of RACs is

$$P_{3d}^{C} = \frac{1}{3}\left(1 + \frac{3}{d} - \frac{1}{d^2}\right). \tag{2}$$

Then we solve the inequality $\frac{1}{3}\left(1 + \frac{1}{\sqrt{d}}\right) > \frac{1}{3}\left(1 + \frac{3}{d} - \frac{1}{d^2}\right)$, we can get

$$\left(\sqrt{d}\right)^3 - 3\left(\sqrt{d}\right)^2 + 1 > 0. \tag{3}$$

It's a cubic function and the zero points are -0.532, 0.653 and 2.880, so when $\sqrt{d} > 2.880$, namely $d \geqslant 9$, $P_{3d}^{QM} > P_{3d}^{C}$ is always right. And for $2 \leqslant d \leqslant 8$, we can find all the subsets of MUBs (when $d = 6$, we use the only 3 bases people know until now) and calculate the corresponding $P_{3d}^{QM}$. We list $P_{3d+}^{QM}$, $P_{3d-}^{QM}$ and $P_{3d}^{C}$ in Table S1.

*R.-H. Miao and Z.-D. Liu contributed equally to this work
†zdliu@ustc.edu.cn
‡synan@hznu.edu.cn
§cfli@ustc.edu.cn

Table S1: $P_{3d+}^{QM}$, $P_{3d-}^{QM}$ and $P_{3d}^{C}$

| $d$ | $P_{3d+}^{QM}$ | $P_{3d-}^{QM}$ | $P_{3d}^{C}$ |
|---|---|---|---|
| 2 | 0.7887 | 0.7887 | 0.7500 |
| 3 | 0.6971 | 0.6971 | 0.6296 |
| 4 | 0.6443 | 0.6443 | 0.5625 |
| 5 | 0.6109 | 0.5964 | 0.5200 |
| 6 | 0.5818 | 0.5818 | 0.4907 |
| 7 | 0.5628 | 0.5628 | 0.4694 |
| 8 | 0.5458 | 0.5458 | 0.4531 |

We find $P_{3d}^{QM} > P_{3d}^{C}$ also standing when $2 \leqslant d \leqslant 8$. So $P_{3d}^{QM} > P_{3d}^{C}$ no matter what $d$ is.

## 2 List of $P_{3d}^{QM}$ in Operational Inequivalence of MUBs in $3^{(d)} \to 1$ QRACs

Here we list the $P_{3d+}^{QM}$ and $P_{3d-}^{QM}$ of $3^{(d)} \to 1$ QRACs when measurement bases are MUBs (shown in Table S2). We calcuate $N$, $P_{3d+}^{QM}$ and $P_{3d-}^{QM}$ of all three-basis-subsets of each $d$ when $d$ is a prime power and $d \leqslant 100$ (such as 4, 25), or $d$ is a prime and $d \leqslant 1000$. We find if $d \equiv 1$ $(mod\ 4)$, $N = 2$, otherwise $N = 1$.

Table S2: $N$, $P_{3d+}^{QM}$ and $P_{3d-}^{QM}$

| $d$ | $N$ | $P_{3d+}^{QM}$ | $P_{3d-}^{QM}$ | $d$ | $N$ | $P_{3d+}^{QM}$ | $P_{3d-}^{QM}$ | $d$ | $N$ | $P_{3d+}^{QM}$ | $P_{3d-}^{QM}$ |
|---|---|---|---|---|---|---|---|---|---|---|---|
| 2 | 1 | 0.788675 | | 3 | 1 | 0.697146 | | 4 | 1 | 0.644338 | |
| 5 | 2 | 0.610855 | 0.596449 | 7 | 1 | 0.562774 | | 8 | 1 | 0.545753 | |
| 9 | 2 | 0.532449 | 0.531297 | 11 | 1 | 0.511553 | | 13 | 2 | 0.499570 | 0.494976 |
| 16 | 1 | 0.478419 | | 17 | 2 | 0.475943 | 0.472029 | 19 | 1 | 0.467949 | |
| 23 | 1 | 0.453727 | | 25 | 2 | 0.450379 | 0.448861 | 27 | 1 | 0.444853 | |
| 29 | 2 | 0.441092 | 0.439367 | 31 | 1 | 0.437380 | | 32 | 1 | 0.435730 | |
| 37 | 2 | 0.428780 | 0.427247 | 41 | 2 | 0.423405 | 0.421591 | 43 | 1 | 0.420914 | |
| 47 | 1 | 0.416312 | | 49 | 2 | 0.415871 | 0.414701 | 53 | 2 | 0.411853 | 0.410980 |
| 59 | 1 | 0.407290 | | 61 | 2 | 0.406941 | 0.405988 | 64 | 1 | 0.403272 | |
| 67 | 1 | 0.402944 | | 71 | 1 | 0.400629 | | 73 | 2 | 0.400419 | 0.399231 |
| 79 | 1 | 0.397391 | | 81 | 2 | 0.397138 | 0.394496 | 83 | 1 | 0.395275 | |
| 89 | 2 | 0.393635 | 0.392777 | 97 | 2 | 0.391254 | 0.390350 | 101 | 2 | 0.389696 | 0.389229 |
| 103 | 1 | 0.389088 | | 107 | 1 | 0.387780 | | 109 | 2 | 0.387871 | 0.387327 |
| 113 | 2 | 0.386621 | 0.385966 | 127 | 1 | 0.383442 | | 131 | 1 | 0.382478 | |
| 137 | 2 | 0.381610 | 0.381069 | 139 | 1 | 0.381219 | | 149 | 2 | 0.379545 | 0.379220 |
| 151 | 1 | 0.379261 | | 157 | 2 | 0.378448 | 0.378100 | 163 | 1 | 0.377444 | |
| 167 | 1 | 0.376698 | | 173 | 2 | 0.376061 | 0.375811 | 179 | 1 | 0.375291 | |
| 181 | 2 | 0.375342 | 0.375019 | 191 | 1 | 0.373929 | | 193 | 2 | 0.374019 | 0.373552 |
| 197 | 2 | 0.373348 | 0.373121 | 199 | 1 | 0.373208 | | 211 | 1 | 0.372051 | |
| 223 | 1 | 0.370909 | | 227 | 1 | 0.370441 | | 229 | 2 | 0.370578 | 0.370324 |
| 233 | 2 | 0.370139 | 0.369823 | 239 | 1 | 0.369547 | | 241 | 2 | 0.369677 | 0.369289 |
| 251 | 1 | 0.368649 | | 257 | 2 | 0.368335 | 0.368054 | 263 | 1 | 0.367799 | |
| 269 | 2 | 0.367515 | 0.367340 | 271 | 1 | 0.367397 | | 277 | 2 | 0.367104 | 0.366902 |
| 281 | 2 | 0.366828 | 0.366548 | 283 | 1 | 0.366619 | | 293 | 2 | 0.366016 | 0.365871 |
| 307 | 1 | 0.365269 | | 311 | 1 | 0.365012 | | 313 | 2 | 0.365107 | 0.364822 |
| 317 | 2 | 0.364759 | 0.364617 | 331 | 1 | 0.364127 | | 337 | 2 | 0.363944 | 0.363674 |
| 347 | 1 | 0.363285 | | 349 | 2 | 0.363374 | 0.363208 | 353 | 2 | 0.363120 | 0.362916 |
| 359 | 1 | 0.362797 | | 367 | 1 | 0.362513 | | 373 | 2 | 0.362359 | 0.362209 |
| 379 | 1 | 0.362079 | | 383 | 1 | 0.361816 | | 389 | 2 | 0.361695 | 0.361568 |
| 397 | 2 | 0.361440 | 0.361304 | 401 | 2 | 0.361293 | 0.361095 | 409 | 2 | 0.361087 | 0.360856 |
| 419 | 1 | 0.360576 | | 421 | 2 | 0.360659 | 0.360516 | 431 | 1 | 0.360192 | |
| 433 | 2 | 0.360271 | 0.360064 | 439 | 1 | 0.360001 | | 443 | 1 | 0.359812 | |
| 449 | 2 | 0.359734 | 0.359557 | 457 | 2 | 0.359549 | 0.359350 | 461 | 2 | 0.359337 | 0.359236 |
| 463 | 1 | 0.359284 | | 467 | 1 | 0.359105 | | 479 | 1 | 0.358787 | |
| 487 | 1 | 0.358626 | | 491 | 1 | 0.358485 | | 499 | 1 | 0.358339 | |
| 503 | 1 | 0.358151 | | 509 | 2 | 0.358069 | 0.357977 | 521 | 2 | 0.357809 | 0.357660 |
| 523 | 1 | 0.357719 | | 541 | 2 | 0.357388 | 0.357278 | 547 | 1 | 0.357181 | |
| 557 | 2 | 0.356953 | 0.356873 | 563 | 1 | 0.356779 | | 569 | 2 | 0.356748 | 0.356608 |

Table S2 (continued)

| $d$ | $N$ | $P_{3d+}^{QM}$ | $P_{3d-}^{QM}$ | $d$ | $N$ | $P_{3d+}^{QM}$ | $P_{3d-}^{QM}$ | $d$ | $N$ | $P_{3d+}^{QM}$ | $P_{3d-}^{QM}$ |
|---|---|---|---|---|---|---|---|---|---|---|---|
| 571 | 1 | 0.356688 | | 577 | 2 | 0.356616 | 0.356462 | 587 | 1 | 0.356293 | |
| 593 | 2 | 0.356233 | 0.356114 | 599 | 1 | 0.356084 | | 601 | 2 | 0.356159 | 0.356001 |
| 607 | 1 | 0.355949 | | 613 | 2 | 0.355891 | 0.355800 | 617 | 2 | 0.355789 | 0.355669 |
| 619 | 1 | 0.355746 | | 631 | 1 | 0.355539 | | 641 | 2 | 0.355379 | 0.355254 |
| 643 | 1 | 0.355302 | | 647 | 1 | 0.355196 | | 653 | 2 | 0.355135 | 0.355065 |
| 659 | 1 | 0.355011 | | 661 | 2 | 0.355059 | 0.354971 | 673 | 2 | 0.354876 | 0.354740 |
| 677 | 2 | 0.354728 | 0.354665 | 683 | 1 | 0.354610 | | 691 | 1 | 0.354534 | |
| 701 | 2 | 0.354381 | 0.354311 | 709 | 2 | 0.354310 | 0.354225 | 719 | 1 | 0.354075 | |
| 727 | 1 | 0.353984 | | 733 | 2 | 0.353930 | 0.353858 | 739 | 1 | 0.353832 | |
| 743 | 1 | 0.353722 | | 751 | 1 | 0.353668 | | 757 | 2 | 0.353611 | 0.353536 |
| 761 | 2 | 0.353536 | 0.353436 | 769 | 2 | 0.353477 | 0.353354 | 773 | 2 | 0.353345 | 0.353289 |
| 787 | 1 | 0.353167 | | 797 | 2 | 0.353041 | 0.352986 | 809 | 2 | 0.352929 | 0.352831 |
| 811 | 1 | 0.352883 | | 821 | 2 | 0.352764 | 0.352705 | 823 | 1 | 0.352737 | |
| 827 | 1 | 0.352651 | | 829 | 2 | 0.352708 | 0.352637 | 839 | 1 | 0.352519 | |
| 853 | 2 | 0.352410 | 0.352348 | 857 | 2 | 0.352346 | 0.352263 | 859 | 1 | 0.352329 | |
| 863 | 1 | 0.352245 | | 877 | 2 | 0.352151 | 0.352089 | 881 | 2 | 0.352098 | 0.352010 |
| 883 | 1 | 0.352061 | | 887 | 1 | 0.351978 | | 907 | 1 | 0.351807 | |
| 911 | 1 | 0.351746 | | 919 | 1 | 0.351697 | | 929 | 2 | 0.351601 | 0.351518 |
| 937 | 2 | 0.351547 | 0.351453 | 941 | 2 | 0.351464 | 0.351415 | 947 | 1 | 0.351380 | |
| 953 | 2 | 0.351361 | 0.351283 | 967 | 1 | 0.351218 | | 971 | 1 | 0.351160 | |
| 977 | 2 | 0.351137 | 0.351061 | 983 | 1 | 0.351038 | | 991 | 1 | 0.351012 | |
| 997 | 2 | 0.350966 | 0.350913 | | | | | | | | |

# 3 Proving MUBs Are Not The Optimal Measurement Bases

We want to find bases that are greater than MUBs and we choose to add noise to MUBs.

From the beginning, we want to create a random noise, we use a random unitary matrix to disturb MUBs. Each basis is transformed by

$$U_{\text{new}}^{r} = SO\left\{U + \delta\left[\text{randn}(d) + \text{randn}(d) * 1\text{i}\right]\right\}. \tag{4}$$

Here $SO$ denotes Schmidt orthogonalization. $U$ represents a basis. $U$ is a $d \times d$ complex matrix joined by $d$ column vectors (each column vector is a quantum state in the basis). $\text{randn}(d)$ is a $d \times d$ real matrix and each element of the matrix obeys the standard normal distribution, $SO\left\{\left[\text{randn}(d) + \text{randn}(d) * 1\text{i}\right]/\sqrt{2}\right\}$ can create a random unitary matrix [1]. $\delta$ is an independent variable that represents the degree of deviation from the MUBs. Actually, we can get some surpass bases using Eq. (4), however because of the randomness, it's difficult to show the result in our paper. So we reselect an easier and more definite way to construct greater bases. Our inspiration comes from reference [2] and we define a new noisy bases

$$U_{\text{new}} = SO(U + \delta\mathbb{I}). \tag{5}$$

Here $\mathbb{I}$ is the identity $d \times d$ matrix. Then we calculate the $P_{3d}^{Q}$ of different $\delta$ and different choice of subsets when $d = 2$, 3, 4, 5, 7, 8, 9, 11, 13, 16, 17, 19, 23, 25, 27, 29 (shown in Fig. S1). We can see when $d = 9$, 16, 17, 23, 25 we can obtain greater bases in this simpler way.

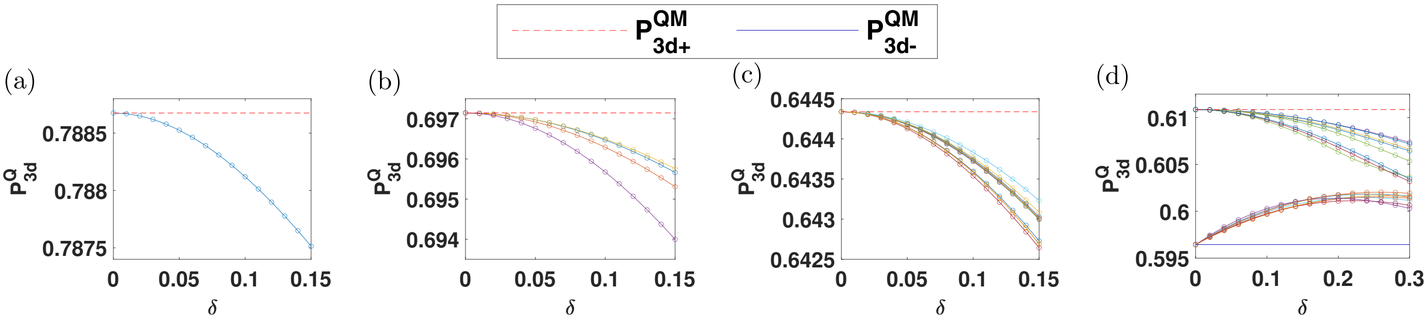


$d = 2$ $d = 3$ $d = 4$ $d = 5$

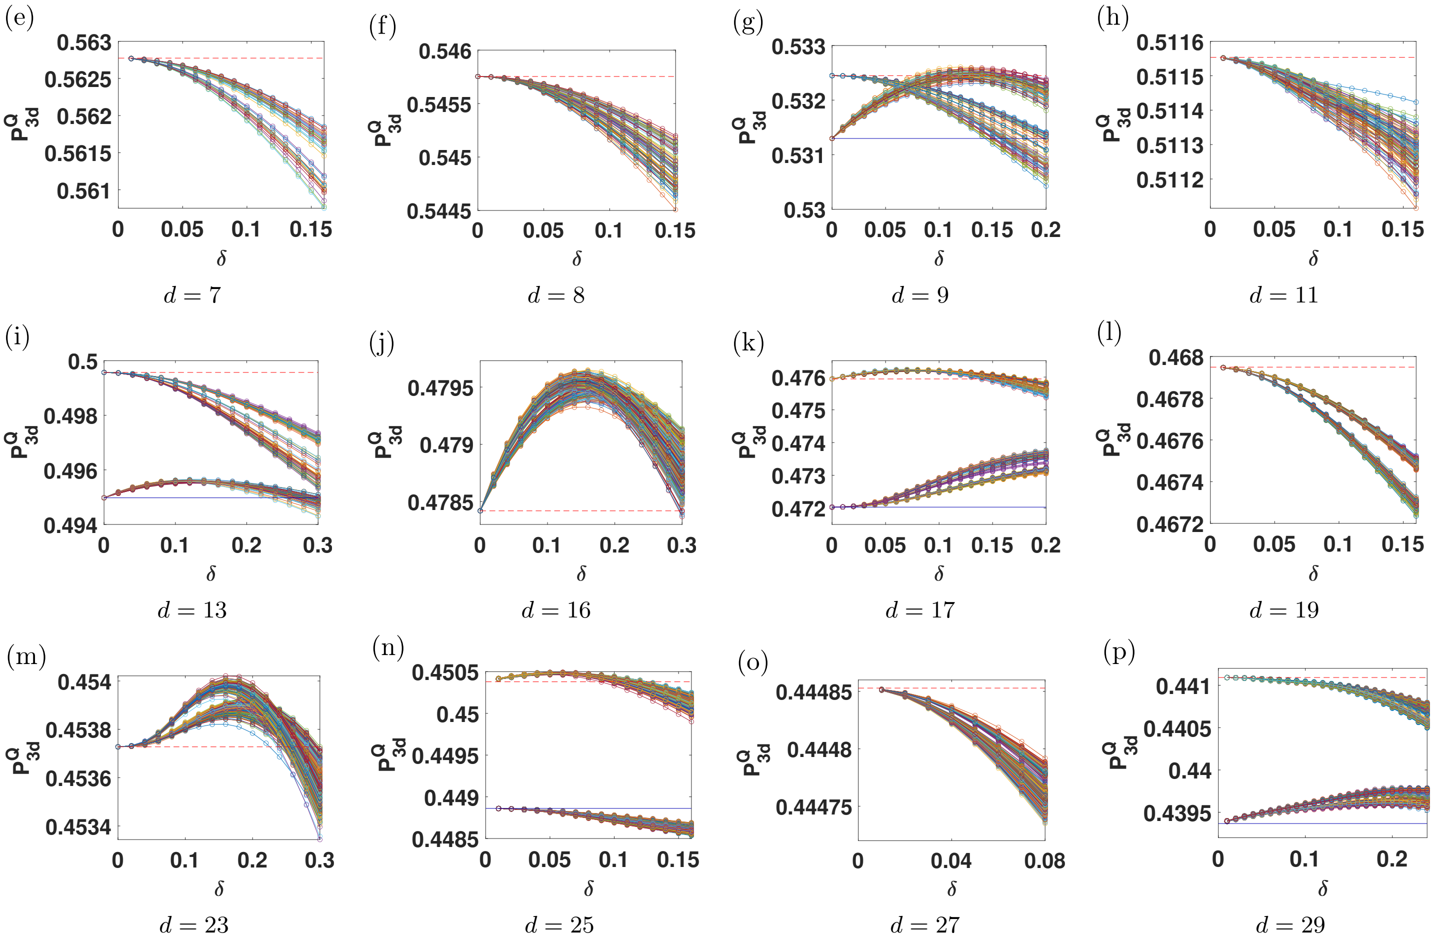


FIG. S1: $P_{3d}^{Q}$ of different $d$, different $\delta$ and different choice of subset. $\delta$ is an independent variable in Eq. (5) that represents the degree of deviation from the MUBs. The red dashed horizontal line (upper or the only horizontal line) and blue solid horizontal line (lower horizontal line) represent $P_{3d+}^{\mathrm{QM}}$ and $P_{3d-}^{\mathrm{QM}}$. Each curved line (colorful, without legend) represents a choice of a three-basis-subset of new bases. The $P_{3d+}^{\mathrm{QM}}$ values for $d = 9$, 16, 17, 23, and 25 can be surpassed.

To show our result clearly, we show the best bases among our calculation numerically when $d = 9$ (shown in Eq. (27), Eq. (28) and Eq. (29) with three decimal places precision). Here $\delta = 0.12$. We can see each basis is a complete orthogonal basis but not mutually unbiased to others.

# 4 Visibility of Laguerre-Gaussian Mode When $d = 11$

Visibility represents the proportion of projecting to the correct state, namely the overlap proportion. For example, the visibility of $\left|\xi_i^{(\mu)}\right\rangle$ is visibility $\left(\left|\xi_i^{(\mu)}\right\rangle\right) = \frac{\mathrm{tr}\left[\rho\left(\left|\xi_i^{(\mu)}\right\rangle\right)\left|\xi_i^{(\mu)}\right\rangle\left\langle\xi_i^{(\mu)}\right|\right]}{\sum_j \mathrm{tr}\left[\rho\left(\left|\xi_i^{(\mu)}\right\rangle\right)\left|\xi_j^{(\mu)}\right\rangle\left\langle\xi_j^{(\mu)}\right|\right]}$, here $\rho\left(\left|\xi_i^{(\mu)}\right\rangle\right)$ represents the state we obtained in experiment after preparation process, and numerator represents the coincidence count when projecting the state we obtained onto state $\left|\xi_i^{(\mu)}\right\rangle$ in experiment, and the denominator represents total counts when projecting the state we obtained onto a orthogonal and complete basis in experiment.

We use both the azimuthal index $l$ and the radial index $p$ of the Laguerre-Gaussian mode. When $d = 11$, we use $|l = 0, \pm 2, \pm 4, \pm 6; p = 0\rangle$ and $|l = \pm 1, \pm 3; p = 2\rangle$ as the basic basis $\left\{\left|\xi_i^{(0)}\right\rangle\right\}$. We use such interlaced $l$ and $p$ because if we only change $p$ without changing $l$, the visibility is unacceptable. So when $p = 0$ we use even $l$ and when $p = 2$ we use odd $l$. We generate each state and measure it with the whole basic basis $\left\{\left|\xi_i^{(0)}\right\rangle\right\}$ when $d = 11$. Shown in Fig. S2, here $\left|\xi_0^{(0)}\right\rangle, \left|\xi_1^{(0)}\right\rangle, \cdots, \left|\xi_6^{(0)}\right\rangle$ match states $|l = 0, 2, -2, 4, -4, 6, -6; p = 0\rangle$, $\left|\xi_7^{(0)}\right\rangle, \left|\xi_8^{(0)}\right\rangle, \cdots, \left|\xi_{10}^{(0)}\right\rangle$ match states $|l = 1, -1, 3, -3; p = 2\rangle$. The visibility of $\left\{\left|\xi_i^{(0)}\right\rangle\right\}$ is larger than 99.25% (namely, 132:1). The worst visibility 99.25% comes in $\left|\xi_{10}^{(0)}\right\rangle$, and the best visibility 99.89% comes in $\left|\xi_0^{(0)}\right\rangle$. This visibility is good enough for our experiment.

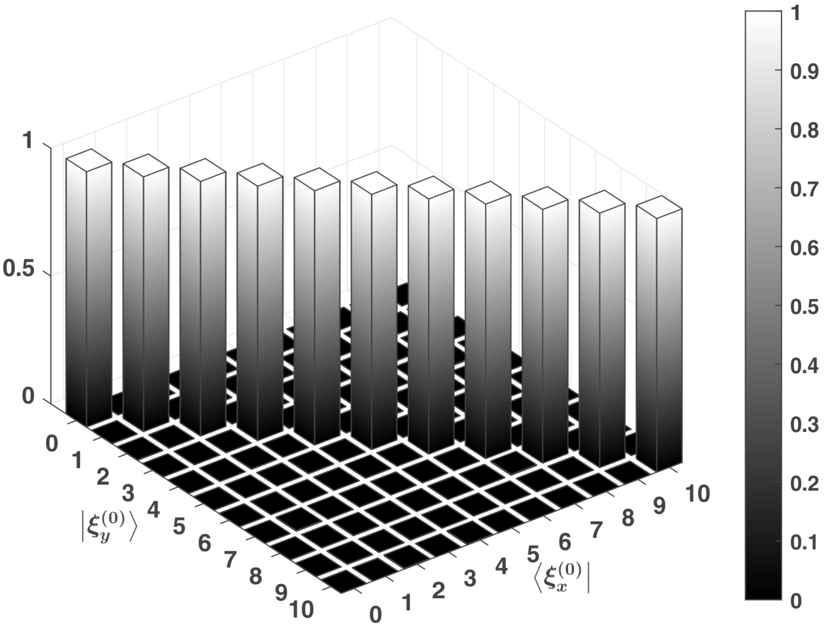


FIG. S2: Visibility of basic basis $\left\{\left|\xi_i^{(0)}\right\rangle\right\}$ when $d = 11$.

## 5 The Bases We Used in The Experiment of $3^{(d)} \to 1$ QRACs

Considering the operational inequivalence of MUBs and the noisy MUBs, we need to choose the bases $\{|c_i\rangle\}$, $\{|e_i\rangle\}$, and $\{|f_i\rangle\}$ carefully. We have introduced how to choose the bases in the paper and now we will show them with three decimal places precision. Here $U$ represents a basis, $U$ is a $d \times d$ complex matrix joined by $d$ column vectors (each column vector is a quantum state in the basis).

$$U_{\{|c_i\rangle\}}(d=2) = \begin{pmatrix} +1.000-0.000\mathrm{i} & +0.000-0.000\mathrm{i} \\ +0.000-0.000\mathrm{i} & +1.000-0.000\mathrm{i} \end{pmatrix}, \tag{6}$$

$$U_{\{|e_i\rangle\}}(d=2) = \begin{pmatrix} +0.707-0.000\mathrm{i} & +0.707-0.000\mathrm{i} \\ +0.707-0.000\mathrm{i} & -0.707+0.000\mathrm{i} \end{pmatrix}, \tag{7}$$

$$U_{\{|f_i\rangle\}}(d=2) = \begin{pmatrix} +0.707-0.000\mathrm{i} & +0.707-0.000\mathrm{i} \\ +0.000+0.707\mathrm{i} & -0.000-0.707\mathrm{i} \end{pmatrix}, \tag{8}$$

$$U_{\{|c_i\rangle\}}(d=3) = \begin{pmatrix} +0.577-0.000\mathrm{i} & +0.577-0.000\mathrm{i} & +0.577-0.000\mathrm{i} \\ +0.577-0.000\mathrm{i} & -0.289+0.500\mathrm{i} & -0.289-0.500\mathrm{i} \\ +0.577-0.000\mathrm{i} & -0.289-0.500\mathrm{i} & -0.289+0.500\mathrm{i} \end{pmatrix}, \tag{9}$$

$$U_{\{|e_i\rangle\}}(d=3) = \begin{pmatrix} +0.577-0.000\mathrm{i} & +0.577-0.000\mathrm{i} & +0.577-0.000\mathrm{i} \\ -0.289+0.500\mathrm{i} & -0.289-0.500\mathrm{i} & +0.577-0.000\mathrm{i} \\ -0.289+0.500\mathrm{i} & +0.577-0.000\mathrm{i} & -0.289-0.500\mathrm{i} \end{pmatrix}, \tag{10}$$

$$U_{\{|f_i\rangle\}}(d=3) = \begin{pmatrix} +0.577-0.000\mathrm{i} & +0.577-0.000\mathrm{i} & +0.577-0.000\mathrm{i} \\ -0.289-0.500\mathrm{i} & +0.577-0.000\mathrm{i} & -0.289+0.500\mathrm{i} \\ -0.289-0.500\mathrm{i} & -0.289+0.500\mathrm{i} & +0.577-0.000\mathrm{i} \end{pmatrix}, \tag{11}$$

$$U_{\{|c_i\rangle\}}(d=4) = \begin{pmatrix} +0.500-0.000\mathrm{i} & +0.500-0.000\mathrm{i} & +0.500-0.000\mathrm{i} & +0.500-0.000\mathrm{i} \\ +0.500-0.000\mathrm{i} & -0.500-0.000\mathrm{i} & +0.500-0.000\mathrm{i} & -0.500-0.000\mathrm{i} \\ +0.500-0.000\mathrm{i} & +0.500-0.000\mathrm{i} & -0.500-0.000\mathrm{i} & -0.500-0.000\mathrm{i} \\ +0.500-0.000\mathrm{i} & -0.500-0.000\mathrm{i} & -0.500-0.000\mathrm{i} & +0.500-0.000\mathrm{i} \end{pmatrix}, \tag{12}$$

$$U_{\{|e_i\rangle\}}(d=4) =$$
$$\begin{pmatrix} +0.500-0.000i & +0.500-0.000i & +0.500-0.000i & +0.500-0.000i \\ +0.000-0.500i & +0.000+0.500i & +0.000-0.500i & +0.000+0.500i \\ +0.000+0.500i & +0.000+0.500i & +0.000-0.500i & +0.000-0.500i \\ +0.500-0.000i & -0.500-0.000i & -0.500-0.000i & +0.500-0.000i \end{pmatrix}, \tag{13}$$

$$U_{\{|f_i\rangle\}}(d=4) =$$
$$\begin{pmatrix} +0.500-0.000i & +0.500-0.000i & +0.500-0.000i & +0.500-0.000i \\ -0.500-0.000i & +0.500-0.000i & -0.500-0.000i & +0.500-0.000i \\ +0.000-0.500i & +0.000-0.500i & +0.000+0.500i & +0.000+0.500i \\ +0.000-0.500i & +0.000+0.500i & +0.000+0.500i & +0.000-0.500i \end{pmatrix}, \tag{14}$$

$$U_{\{|c_i\rangle\}}(d=5) =$$
$$\begin{pmatrix} +0.447-0.000i & +0.447-0.000i & +0.447-0.000i & +0.447-0.000i & +0.447-0.000i \\ +0.447-0.000i & +0.138+0.425i & -0.362+0.263i & -0.362-0.263i & +0.138-0.425i \\ +0.447-0.000i & -0.362+0.263i & +0.138-0.425i & +0.138+0.425i & -0.362-0.263i \\ +0.447-0.000i & -0.362-0.263i & +0.138+0.425i & +0.138-0.425i & -0.362+0.263i \\ +0.447-0.000i & +0.138-0.425i & -0.362-0.263i & -0.362+0.263i & +0.138+0.425i \end{pmatrix}, \tag{15}$$

$$U_{\{|e_i\rangle\}}(d=5) =$$
$$\begin{pmatrix} +0.447-0.000i & +0.447-0.000i & +0.447-0.000i & +0.447-0.000i & +0.447-0.000i \\ +0.138+0.425i & -0.362+0.263i & -0.362-0.263i & +0.138-0.425i & +0.447-0.000i \\ +0.138-0.425i & +0.138+0.425i & -0.362-0.263i & +0.447-0.000i & -0.362+0.263i \\ +0.138-0.425i & -0.362+0.263i & +0.447-0.000i & -0.362-0.263i & +0.138+0.425i \\ +0.138+0.425i & +0.447-0.000i & +0.138-0.425i & -0.362-0.263i & -0.362+0.263i \end{pmatrix}, \tag{16}$$

$$U_{\{|f_i\rangle\}}(d=5) =$$
$$\begin{pmatrix} +0.447-0.000i & +0.447-0.000i & +0.447-0.000i & +0.447-0.000i & +0.447-0.000i \\ -0.362-0.263i & +0.138-0.425i & +0.447-0.000i & +0.138+0.425i & -0.362+0.263i \\ -0.362+0.263i & +0.138-0.425i & +0.138+0.425i & -0.362-0.263i & +0.447-0.000i \\ -0.362+0.263i & +0.447-0.000i & -0.362-0.263i & +0.138+0.425i & +0.138-0.425i \\ -0.362-0.263i & -0.362+0.263i & +0.138+0.425i & +0.447-0.000i & +0.138-0.425i \end{pmatrix}, \tag{17}$$

$$U_{\{|c_i\rangle\}}(d=6) =$$
$$\begin{pmatrix} +1.000-0.000i & +0.000-0.000i & +0.000-0.000i & +0.000-0.000i & +0.000-0.000i & +0.000-0.000i \\ +0.000-0.000i & +1.000-0.000i & +0.000-0.000i & +0.000-0.000i & +0.000-0.000i & +0.000-0.000i \\ +0.000-0.000i & +0.000-0.000i & +1.000-0.000i & +0.000-0.000i & +0.000-0.000i & +0.000-0.000i \\ +0.000-0.000i & +0.000-0.000i & +0.000-0.000i & +1.000-0.000i & +0.000-0.000i & +0.000-0.000i \\ +0.000-0.000i & +0.000-0.000i & +0.000-0.000i & +0.000-0.000i & +1.000-0.000i & +0.000-0.000i \\ +0.000-0.000i & +0.000-0.000i & +0.000-0.000i & +0.000-0.000i & +0.000-0.000i & +1.000-0.000i \end{pmatrix}, \tag{18}$$

$$U_{\{|e_i\rangle\}}(d=6) =$$
$$\begin{pmatrix} +0.408-0.000i & +0.408-0.000i & +0.408-0.000i & +0.408-0.000i & +0.408-0.000i & +0.408-0.000i \\ +0.408-0.000i & +0.204+0.354i & -0.204+0.354i & -0.408+0.000i & -0.204-0.354i & +0.204-0.354i \\ +0.408-0.000i & -0.204+0.354i & -0.204-0.354i & +0.408-0.000i & -0.204+0.354i & -0.204-0.354i \\ +0.408-0.000i & -0.408+0.000i & +0.408-0.000i & -0.408+0.000i & +0.408-0.000i & -0.408+0.000i \\ +0.408-0.000i & -0.204-0.354i & -0.204+0.354i & +0.408-0.000i & -0.204-0.354i & -0.204+0.354i \\ +0.408-0.000i & +0.204-0.354i & -0.204-0.354i & -0.408+0.000i & -0.204+0.354i & +0.204+0.354i \end{pmatrix}, \tag{19}$$

$$U_{\{|f_i\rangle\}}(d=6) =$$
$$\begin{pmatrix} +0.408-0.000i & +0.408-0.000i & +0.408-0.000i & +0.408-0.000i & +0.408-0.000i & +0.408-0.000i \\ +0.354+0.204i & +0.000+0.408i & -0.354+0.204i & -0.354-0.204i & -0.000-0.408i & +0.354-0.204i \\ -0.204+0.354i & -0.204-0.354i & +0.408-0.000i & -0.204+0.354i & -0.204-0.354i & +0.408-0.000i \\ -0.000-0.408i & +0.000+0.408i & -0.000-0.408i & +0.000+0.408i & -0.000-0.408i & +0.000+0.408i \\ -0.204+0.354i & +0.408-0.000i & -0.204-0.354i & -0.204+0.354i & +0.408-0.000i & -0.204-0.354i \\ +0.354+0.204i & +0.354-0.204i & -0.000-0.408i & -0.354-0.204i & -0.354+0.204i & +0.000+0.408i \end{pmatrix}, \tag{20}$$

$$U_{\{|c_i\rangle\}}(d=7) =$$
$$\begin{pmatrix} +0.378-0.000i & +0.378-0.000i & +0.378-0.000i & +0.378-0.000i & +0.378-0.000i & +0.378-0.000i & +0.378-0.000i \\ +0.378-0.000i & +0.236+0.296i & -0.084+0.368i & -0.341+0.164i & -0.341-0.164i & -0.084-0.368i & +0.236-0.296i \\ +0.378-0.000i & -0.084+0.368i & -0.341-0.164i & +0.236-0.296i & +0.236+0.296i & -0.341+0.164i & -0.084-0.368i \\ +0.378-0.000i & -0.341+0.164i & +0.236-0.296i & -0.084+0.368i & -0.084-0.368i & +0.236+0.296i & -0.341-0.164i \\ +0.378-0.000i & -0.341-0.164i & +0.236+0.296i & -0.084-0.368i & -0.084+0.368i & +0.236-0.296i & -0.341+0.164i \\ +0.378-0.000i & -0.084-0.368i & -0.341+0.164i & +0.236+0.296i & +0.236-0.296i & -0.341-0.164i & -0.084+0.368i \\ +0.378-0.000i & +0.236-0.296i & -0.084-0.368i & -0.341-0.164i & -0.341+0.164i & -0.084+0.368i & +0.236+0.296i \end{pmatrix}, \tag{21}$$

$$U_{\{|e_i\rangle\}}(d=7) =$$
$$\begin{pmatrix} +0.378-0.000i & +0.378-0.000i & +0.378-0.000i & +0.378-0.000i & +0.378-0.000i & +0.378-0.000i & +0.378-0.000i \\ +0.236+0.296i & -0.084+0.368i & -0.341+0.164i & -0.341-0.164i & -0.084-0.368i & +0.236-0.296i & +0.378-0.000i \\ -0.341-0.164i & +0.236-0.296i & +0.236+0.296i & -0.341+0.164i & -0.084-0.368i & +0.378-0.000i & -0.084+0.368i \\ -0.084+0.368i & -0.084-0.368i & +0.236+0.296i & -0.341-0.164i & +0.378-0.000i & -0.341+0.164i & +0.236-0.296i \\ -0.084+0.368i & +0.236-0.296i & -0.341+0.164i & +0.378-0.000i & -0.341-0.164i & +0.236+0.296i & -0.084-0.368i \\ -0.341-0.164i & -0.084+0.368i & +0.378-0.000i & -0.084-0.368i & -0.341+0.164i & +0.236+0.296i & +0.236-0.296i \\ +0.236+0.296i & +0.378-0.000i & +0.236-0.296i & -0.084-0.368i & -0.341-0.164i & -0.341+0.164i & -0.084+0.368i \end{pmatrix}, \tag{22}$$

$$U_{\{|f_i\rangle\}}(d=7) =$$
$$\begin{pmatrix} +0.378-0.000i & +0.378-0.000i & +0.378-0.000i & +0.378-0.000i & +0.378-0.000i & +0.378-0.000i & +0.378-0.000i \\ -0.084+0.368i & -0.341+0.164i & -0.341-0.164i & -0.084-0.368i & +0.236-0.296i & +0.378-0.000i & +0.236+0.296i \\ +0.236+0.296i & -0.341+0.164i & -0.084-0.368i & +0.378-0.000i & -0.084+0.368i & -0.341-0.164i & +0.236-0.296i \\ -0.341-0.164i & +0.378-0.000i & -0.341+0.164i & +0.236-0.296i & -0.084+0.368i & -0.084-0.368i & +0.236+0.296i \\ -0.341-0.164i & +0.236+0.296i & -0.084-0.368i & -0.084+0.368i & +0.236-0.296i & -0.341+0.164i & +0.378-0.000i \\ +0.236+0.296i & +0.236-0.296i & -0.341-0.164i & -0.084+0.368i & +0.378-0.000i & -0.084-0.368i & -0.341+0.164i \\ -0.084+0.368i & +0.236+0.296i & +0.378-0.000i & +0.236-0.296i & -0.084-0.368i & -0.341-0.164i & -0.341+0.164i \end{pmatrix}, \tag{23}$$

$$U_{\{|c_i\rangle\}}(d=8) =$$

$$\begin{pmatrix}
+0.354-0.000i & +0.354-0.000i & +0.354-0.000i & +0.354-0.000i & +0.354-0.000i & +0.354-0.000i & +0.354-0.000i & +0.354-0.000i \\
+0.354-0.000i & -0.354-0.000i & +0.354-0.000i & -0.354-0.000i & +0.354-0.000i & -0.354-0.000i & +0.354-0.000i & -0.354-0.000i \\
+0.354-0.000i & +0.354-0.000i & +0.354-0.000i & +0.354-0.000i & -0.354-0.000i & -0.354-0.000i & -0.354-0.000i & -0.354-0.000i \\
+0.354-0.000i & -0.354-0.000i & +0.354-0.000i & -0.354-0.000i & -0.354-0.000i & +0.354-0.000i & -0.354-0.000i & +0.354-0.000i \\
+0.354-0.000i & +0.354-0.000i & -0.354-0.000i & -0.354-0.000i & +0.354-0.000i & +0.354-0.000i & -0.354-0.000i & -0.354-0.000i \\
+0.354-0.000i & -0.354-0.000i & -0.354-0.000i & +0.354-0.000i & +0.354-0.000i & -0.354-0.000i & -0.354-0.000i & +0.354-0.000i \\
+0.354-0.000i & +0.354-0.000i & -0.354-0.000i & -0.354-0.000i & -0.354-0.000i & -0.354-0.000i & +0.354-0.000i & +0.354-0.000i \\
+0.354-0.000i & -0.354-0.000i & -0.354-0.000i & +0.354-0.000i & -0.354-0.000i & +0.354-0.000i & +0.354-0.000i & -0.354-0.000i
\end{pmatrix}, \quad (24)$$

$$U_{\{|e_i\rangle\}}(d=8) =$$

$$\begin{pmatrix}
+0.354-0.000i & +0.354-0.000i & +0.354-0.000i & +0.354-0.000i & +0.354-0.000i & +0.354-0.000i & +0.354-0.000i & +0.354-0.000i \\
+0.000-0.354i & +0.000+0.354i & +0.000-0.354i & +0.000+0.354i & +0.000-0.354i & +0.000+0.354i & +0.000-0.354i & +0.000+0.354i \\
+0.354-0.000i & +0.354-0.000i & +0.354-0.000i & +0.354-0.000i & -0.354-0.000i & -0.354-0.000i & -0.354-0.000i & -0.354-0.000i \\
+0.000-0.354i & +0.000+0.354i & +0.000-0.354i & +0.000+0.354i & +0.000+0.354i & +0.000-0.354i & +0.000+0.354i & +0.000-0.354i \\
-0.354-0.000i & -0.354-0.000i & +0.354-0.000i & +0.354-0.000i & -0.354-0.000i & -0.354-0.000i & +0.354-0.000i & +0.354-0.000i \\
+0.000+0.354i & +0.000-0.354i & +0.000-0.354i & +0.000+0.354i & +0.000+0.354i & +0.000-0.354i & +0.000-0.354i & +0.000+0.354i \\
+0.354-0.000i & +0.354-0.000i & -0.354-0.000i & -0.354-0.000i & -0.354-0.000i & -0.354-0.000i & +0.354-0.000i & +0.354-0.000i \\
+0.000-0.354i & +0.000+0.354i & +0.000+0.354i & +0.000-0.354i & +0.000+0.354i & +0.000-0.354i & +0.000-0.354i & +0.000+0.354i
\end{pmatrix}, \quad (25)$$

$$U_{\{|f_i\rangle\}}(d=8) =$$

$$\begin{pmatrix}
+0.354-0.000i & +0.354-0.000i & +0.354-0.000i & +0.354-0.000i & +0.354-0.000i & +0.354-0.000i & +0.354-0.000i & +0.354-0.000i \\
-0.354-0.000i & +0.354-0.000i & -0.354-0.000i & +0.354-0.000i & -0.354-0.000i & +0.354-0.000i & -0.354-0.000i & +0.354-0.000i \\
+0.000+0.354i & +0.000+0.354i & +0.000+0.354i & +0.000+0.354i & +0.000-0.354i & +0.000-0.354i & +0.000-0.354i & +0.000-0.354i \\
+0.000-0.354i & +0.000+0.354i & +0.000-0.354i & +0.000+0.354i & +0.000+0.354i & +0.000-0.354i & +0.000+0.354i & +0.000-0.354i \\
+0.000+0.354i & +0.000+0.354i & +0.000-0.354i & +0.000-0.354i & +0.000+0.354i & +0.000+0.354i & +0.000-0.354i & +0.000-0.354i \\
+0.000+0.354i & +0.000-0.354i & +0.000-0.354i & +0.000+0.354i & +0.000+0.354i & +0.000-0.354i & +0.000-0.354i & +0.000+0.354i \\
-0.354-0.000i & -0.354-0.000i & +0.354-0.000i & +0.354-0.000i & +0.354-0.000i & +0.354-0.000i & -0.354-0.000i & -0.354-0.000i \\
-0.354-0.000i & +0.354-0.000i & +0.354-0.000i & -0.354-0.000i & +0.354-0.000i & -0.354-0.000i & -0.354-0.000i & +0.354-0.000i
\end{pmatrix}, \quad (26)$$

$$U_{\{|c_i\rangle\}}(d=9) =$$

$$\begin{pmatrix}
+0.433-0.000i & +0.305-0.000i & +0.320-0.000i & +0.317-0.000i & +0.332-0.000i & +0.283-0.000i & +0.323-0.000i & +0.315-0.000i & +0.350-0.000i \\
+0.319-0.000i & -0.072-0.293i & -0.198+0.280i & -0.196-0.277i & -0.205+0.265i & +0.322+0.000i & -0.181+0.308i & +0.337+0.012i & -0.175-0.295i \\
+0.319-0.000i & -0.194+0.293i & -0.081-0.280i & -0.196+0.277i & -0.205-0.265i & +0.322-0.000i & -0.181-0.308i & +0.337-0.012i & -0.175+0.295i \\
+0.319-0.000i & -0.194-0.293i & -0.204+0.280i & +0.394-0.000i & -0.184-0.278i & -0.157+0.285i & +0.240-0.002i & -0.157-0.289i & -0.175+0.295i \\
+0.319-0.000i & -0.194+0.293i & -0.204-0.280i & -0.202-0.277i & +0.385-0.013i & -0.157+0.285i & -0.178+0.306i & -0.174-0.277i & +0.226+0.000i \\
+0.319-0.000i & +0.314-0.000i & +0.329-0.000i & -0.154+0.277i & -0.161+0.290i & -0.136+0.318i & -0.157-0.272i & -0.274-0.265i & -0.175-0.295i \\
+0.319-0.000i & -0.194+0.293i & -0.204-0.280i & +0.279-0.000i & -0.189+0.278i & -0.161-0.285i & +0.363+0.002i & -0.157+0.289i & -0.175-0.295i \\
+0.319-0.000i & +0.314-0.000i & +0.329-0.000i & -0.154-0.277i & -0.161-0.290i & -0.259-0.318i & -0.161+0.272i & -0.159+0.265i & -0.175+0.295i \\
+0.319-0.000i & -0.194-0.293i & -0.204+0.280i & -0.202+0.277i & +0.269+0.013i & -0.161-0.285i & -0.184-0.306i & -0.179+0.277i & +0.348-0.000i
\end{pmatrix}, \quad (27)$$

$$U_{\{|e_i\rangle\}}(d=9) =$$

$$\begin{pmatrix}
+0.433-0.000i & +0.330-0.015i & +0.304-0.013i & +0.319-0.014i & +0.309-0.019i & +0.363+0.043i & +0.315+0.012i & +0.294+0.032i & +0.302-0.033i \\
-0.159-0.276i & -0.053+0.303i & +0.337-0.014i & -0.207+0.319i & +0.372-0.015i & -0.136-0.265i & +0.355+0.012i & -0.181-0.258i & -0.122+0.278i \\
-0.159-0.276i & +0.332+0.011i & -0.081+0.303i & +0.354-0.015i & -0.160+0.265i & -0.183-0.269i & -0.185+0.306i & -0.136-0.284i & +0.368-0.005i \\
-0.159-0.276i & -0.175+0.303i & +0.347-0.014i & -0.091-0.269i & -0.157+0.291i & +0.324+0.043i & -0.165-0.318i & -0.200+0.313i & +0.302+0.033i \\
-0.159+0.276i & -0.157-0.293i & +0.364+0.024i & +0.314-0.015i & -0.074+0.271i & -0.161-0.306i & -0.107-0.278i & +0.365-0.014i & -0.180+0.321i \\
-0.159+0.276i & -0.157+0.293i & -0.144+0.270i & -0.152-0.304i & -0.157-0.293i & -0.119-0.302i & +0.383-0.018i & +0.291+0.038i & +0.360-0.000i \\
-0.159-0.276i & +0.332+0.011i & -0.203+0.303i & -0.145-0.309i & +0.351-0.000i & -0.168+0.330i & -0.114-0.283i & +0.306+0.021i & -0.122+0.278i \\
-0.159+0.276i & -0.157+0.293i & -0.144+0.270i & +0.357-0.010i & +0.351-0.024i & +0.289-0.024i & -0.152-0.279i & -0.171-0.305i & -0.180-0.321i \\
-0.159+0.276i & +0.350+0.000i & -0.185-0.294i & -0.127-0.269i & -0.196+0.292i & +0.345+0.013i & +0.295-0.023i & -0.173-0.331i & -0.128+0.283i
\end{pmatrix}, \quad (28)$$

$$U_{\{|f_i\rangle\}}(d=9) =$$

$$\begin{pmatrix}
+0.433-0.000i & +0.311+0.014i & +0.323+0.014i & +0.319+0.014i & +0.309+0.019i & +0.307-0.043i & +0.318-0.007i & +0.350-0.030i & +0.302+0.033i \\
-0.159+0.276i & +0.428-0.010i & -0.149-0.287i & +0.295-0.021i & -0.157-0.267i & -0.151+0.284i & -0.130-0.274i & -0.163+0.267i & +0.367+0.004i \\
-0.159+0.276i & -0.165-0.286i & +0.422-0.021i & -0.147-0.283i & +0.370+0.016i & -0.175+0.250i & +0.295-0.044i & -0.145+0.277i & -0.121-0.278i \\
-0.159+0.276i & +0.313-0.010i & -0.153-0.287i & -0.083+0.273i & +0.351+0.003i & -0.200-0.309i & -0.170+0.315i & +0.305-0.060i & -0.180-0.312i \\
-0.159-0.276i & +0.330+0.000i & -0.135+0.276i & -0.188+0.304i & -0.074-0.295i & +0.340+0.019i & +0.353-0.013i & -0.144+0.279i & -0.187-0.317i \\
-0.159-0.276i & -0.148-0.276i & -0.153-0.287i & +0.357+0.010i & +0.351+0.024i & +0.348+0.020i & -0.152+0.279i & -0.201+0.289i & -0.122+0.286i \\
-0.159+0.276i & -0.165-0.286i & +0.307-0.021i & -0.152+0.304i & -0.157-0.294i & +0.325-0.009i & -0.104+0.286i & -0.171-0.334i & +0.360+0.000i \\
-0.159-0.276i & -0.148-0.276i & -0.153-0.287i & -0.152+0.304i & -0.157+0.293i & -0.209+0.251i & +0.380+0.024i & +0.350+0.035i & +0.302+0.034i \\
-0.159-0.276i & -0.148+0.276i & +0.325+0.010i & +0.375-0.021i & -0.196-0.268i & -0.133+0.324i & -0.165+0.315i & +0.311+0.015i & -0.121-0.287i
\end{pmatrix}, \quad (29)$$

$$U_{\{|c_i\rangle\}}(d=11) =$$

$$\begin{pmatrix}
+0.302-0.000i & +0.302-0.000i & +0.302-0.000i & +0.302-0.000i & +0.302-0.000i & +0.302-0.000i & +0.302-0.000i & +0.302-0.000i & +0.302-0.000i & +0.302-0.000i & +0.302-0.000i \\
+0.302-0.000i & +0.254+0.163i & +0.125+0.274i & -0.043+0.298i & -0.197+0.228i & -0.289+0.085i & -0.289-0.085i & -0.197-0.228i & -0.043-0.298i & +0.125-0.274i & +0.254-0.163i \\
+0.302-0.000i & +0.125+0.274i & -0.197+0.228i & -0.289-0.085i & -0.043-0.298i & +0.254-0.163i & +0.254+0.163i & -0.043+0.298i & -0.289+0.085i & -0.197-0.228i & +0.125-0.274i \\
+0.302-0.000i & -0.043+0.298i & -0.289-0.085i & +0.125-0.274i & +0.254+0.163i & -0.197+0.228i & -0.197-0.228i & +0.254-0.163i & +0.125+0.274i & -0.289+0.085i & -0.043-0.298i \\
+0.302-0.000i & -0.197+0.228i & -0.043-0.298i & +0.254+0.163i & -0.289+0.085i & +0.125-0.274i & +0.125+0.274i & -0.289-0.085i & +0.254-0.163i & -0.043+0.298i & -0.197-0.228i \\
+0.302-0.000i & -0.289+0.085i & +0.254-0.163i & -0.197+0.228i & +0.125-0.274i & -0.043+0.298i & -0.043-0.298i & +0.125+0.274i & -0.197-0.228i & +0.254+0.163i & -0.289-0.085i \\
+0.302-0.000i & -0.289-0.085i & +0.254+0.163i & -0.197-0.228i & +0.125+0.274i & -0.043-0.298i & -0.043+0.298i & +0.125-0.274i & -0.197+0.228i & +0.254-0.163i & -0.289+0.085i \\
+0.302-0.000i & -0.197-0.228i & -0.043+0.298i & +0.254-0.163i & -0.289-0.085i & +0.125+0.274i & +0.125-0.274i & -0.289+0.085i & +0.254+0.163i & -0.043-0.298i & -0.197+0.228i \\
+0.302-0.000i & -0.043-0.298i & -0.289+0.085i & +0.125+0.274i & +0.254-0.163i & -0.197-0.228i & -0.197+0.228i & +0.254+0.163i & +0.125-0.274i & -0.289-0.085i & -0.043+0.298i \\
+0.302-0.000i & +0.125-0.274i & -0.197-0.228i & -0.289+0.085i & -0.043+0.298i & +0.254+0.163i & +0.254-0.163i & -0.043-0.298i & -0.289-0.085i & -0.197+0.228i & +0.125+0.274i \\
+0.302-0.000i & +0.254-0.163i & +0.125-0.274i & -0.043-0.298i & -0.197-0.228i & -0.289-0.085i & -0.289+0.085i & -0.197+0.228i & -0.043+0.298i & +0.125+0.274i & +0.254+0.163i
\end{pmatrix}, \quad (30)$$

$$U_{\{|e_i\rangle\}}(d=11) =$$

$$\begin{pmatrix}
+0.302-0.000i & +0.302-0.000i & +0.302-0.000i & +0.302-0.000i & +0.302-0.000i & +0.302-0.000i & +0.302-0.000i & +0.302-0.000i & +0.302-0.000i & +0.302-0.000i & +0.302-0.000i \\
+0.254+0.163i & +0.125+0.274i & -0.043+0.298i & -0.197+0.228i & -0.289+0.085i & -0.289-0.085i & -0.197-0.228i & -0.043-0.298i & +0.125-0.274i & +0.254-0.163i & +0.302-0.000i \\
-0.197+0.228i & -0.289-0.085i & -0.043-0.298i & +0.254-0.163i & +0.254+0.163i & -0.043+0.298i & -0.289+0.085i & -0.197-0.228i & +0.125-0.274i & +0.302-0.000i & +0.125+0.274i \\
+0.125-0.274i & +0.254+0.163i & -0.197+0.228i & -0.197-0.228i & +0.254-0.163i & +0.125+0.274i & -0.289+0.085i & -0.043-0.298i & +0.302-0.000i & -0.043+0.298i & -0.289-0.085i \\
-0.289+0.085i & +0.125-0.274i & +0.125+0.274i & -0.289-0.085i & +0.254-0.163i & -0.043+0.298i & -0.197-0.228i & +0.302-0.000i & -0.197+0.228i & -0.043-0.298i & +0.254+0.163i \\
-0.043+0.298i & -0.043-0.298i & +0.125+0.274i & -0.197-0.228i & +0.254+0.163i & -0.289-0.085i & +0.302-0.000i & -0.289+0.085i & +0.254-0.163i & -0.197+0.228i & +0.125-0.274i \\
-0.043+0.298i & +0.125-0.274i & -0.197+0.228i & +0.254-0.163i & -0.289+0.085i & +0.302-0.000i & -0.289-0.085i & +0.254+0.163i & -0.197-0.228i & +0.125+0.274i & -0.043-0.298i \\
-0.289+0.085i & +0.254+0.163i & -0.043-0.298i & -0.197+0.228i & +0.302-0.000i & -0.197-0.228i & -0.043+0.298i & +0.254-0.163i & -0.289-0.085i & +0.125+0.274i & +0.125-0.274i \\
+0.125-0.274i & -0.289-0.085i & -0.043+0.298i & +0.302-0.000i & -0.043-0.298i & -0.289+0.085i & +0.125+0.274i & +0.254-0.163i & -0.197-0.228i & -0.197+0.228i & +0.254+0.163i \\
-0.197+0.228i & +0.125+0.274i & +0.302-0.000i & +0.125-0.274i & -0.197-0.228i & -0.289+0.085i & -0.043+0.298i & +0.254+0.163i & +0.254-0.163i & -0.043-0.298i & -0.289-0.085i \\
+0.254+0.163i & +0.302-0.000i & +0.254-0.163i & +0.125-0.274i & -0.043-0.298i & -0.197-0.228i & -0.289-0.085i & -0.289+0.085i & -0.197+0.228i & -0.043+0.298i & +0.125+0.274i
\end{pmatrix}, \quad (31)$$

$$U_{\{|f_i\rangle\}}(d=11) =$$

$$\begin{pmatrix}
+0.302-0.000i & +0.302-0.000i & +0.302-0.000i & +0.302-0.000i & +0.302-0.000i & +0.302-0.000i & +0.302-0.000i & +0.302-0.000i & +0.302-0.000i & +0.302-0.000i & +0.302-0.000i \\
+0.125+0.274i & -0.043+0.298i & -0.197+0.228i & -0.289+0.085i & -0.289-0.085i & -0.197-0.228i & -0.043-0.298i & +0.125-0.274i & +0.254-0.163i & +0.302-0.000i & +0.254+0.163i \\
-0.043-0.298i & +0.254-0.163i & +0.254+0.163i & -0.043+0.298i & -0.289+0.085i & -0.197-0.228i & +0.125-0.274i & +0.302-0.000i & +0.125+0.274i & -0.197+0.228i & -0.289-0.085i \\
-0.197-0.228i & +0.254-0.163i & +0.125+0.274i & -0.289+0.085i & -0.043-0.298i & +0.302-0.000i & -0.043+0.298i & -0.289-0.085i & +0.125-0.274i & +0.254+0.163i & -0.197+0.228i \\
+0.254-0.163i & -0.043+0.298i & -0.197-0.228i & +0.302-0.000i & -0.197+0.228i & -0.043-0.298i & +0.254+0.163i & -0.289+0.085i & +0.125-0.274i & +0.125+0.274i & -0.289-0.085i \\
-0.289-0.085i & +0.302-0.000i & -0.289+0.085i & +0.254-0.163i & -0.197+0.228i & +0.125-0.274i & -0.043+0.298i & -0.043-0.298i & +0.125+0.274i & -0.197-0.228i & +0.254+0.163i \\
-0.289-0.085i & +0.254+0.163i & -0.197-0.228i & +0.125+0.274i & -0.043-0.298i & -0.043+0.298i & +0.125-0.274i & -0.197+0.228i & +0.254-0.163i & -0.289+0.085i & +0.302-0.000i \\
+0.254-0.163i & -0.289-0.085i & +0.125+0.274i & +0.125-0.274i & -0.289+0.085i & +0.254+0.163i & -0.043-0.298i & -0.197+0.228i & +0.302-0.000i & -0.197-0.228i & -0.043+0.298i \\
-0.197-0.228i & -0.197+0.228i & +0.254+0.163i & +0.125-0.274i & -0.289-0.085i & -0.043+0.298i & +0.302-0.000i & -0.043-0.298i & -0.289+0.085i & +0.125+0.274i & +0.254-0.163i \\
-0.043-0.298i & -0.289-0.085i & -0.197+0.228i & +0.125+0.274i & +0.302-0.000i & +0.125-0.274i & -0.197-0.228i & -0.289+0.085i & -0.043+0.298i & +0.254+0.163i & +0.254-0.163i \\
+0.125+0.274i & +0.254+0.163i & +0.302-0.000i & +0.254-0.163i & +0.125-0.274i & -0.043-0.298i & -0.197-0.228i & -0.289-0.085i & -0.289+0.085i & -0.197+0.228i & -0.043+0.298i
\end{pmatrix}. \quad (32)$$

# 6 The Experimental Results of QRACs

Here we will show the maximum success probabilities of both theory and experiment (with standard deviations), of both QRACs and RACs and for both $2^{(d)} \to 1$ and $3^{(d)} \to 1$.

Table S3: Experimental results of $2^{(d)} \to 1$ QRACs

| $d$ | $P^Q_{2d}$(Theory) | $P^Q_{2d}$(Experiment) | $P^C_{2d}$(Theory) | $P^C_{2d}$(Experiment) |
|---|---|---|---|---|
| 2 | 0.8536 | 0.8530±0.0018 | 0.7500 | 0.7494±0.0001 |
| 3 | 0.7887 | 0.7810±0.0032 | 0.6667 | 0.6660±0.0001 |
| 4 | 0.7500 | 0.7455±0.0020 | 0.6250 | 0.6241±0.0001 |
| 5 | 0.7236 | 0.7225±0.0025 | 0.6000 | 0.5991±0.0002 |
| 6 | 0.7041 | 0.6970±0.0018 | 0.5833 | 0.5817±0.0002 |
| 7 | 0.6890 | 0.6711±0.0036 | 0.5714 | 0.5699±0.0001 |
| 8 | 0.6768 | 0.6614±0.0023 | 0.5625 | 0.5599±0.0001 |
| 9 | 0.6667 | 0.6654±0.0016 | 0.5556 | 0.5537±0.0002 |
| 11 | 0.6508 | 0.6469±0.0017 | 0.5455 | 0.5436±0.0001 |

Table S4: Experimental results of $3^{(d)} \to 1$ QRACs

| $d$ | $P^Q_{3d}$(Theory) | $P^Q_{3d}$(Experiment) | $P^C_{3d}$(Theory) | $P^C_{3d}$(Experiment) |
|---|---|---|---|---|
| 2 | 0.7887 | 0.7870±0.0011 | 0.7500 | 0.7494±0.0001 |
| 3 | 0.6971 | 0.6845±0.0009 | 0.6296 | 0.6290±0.0001 |
| 4 | 0.6443 | 0.6374±0.0014 | 0.5625 | 0.5617±0.0001 |
| 5 | 0.6109 | 0.6004±0.0007 | 0.5200 | 0.5193±0.0001 |
| 6 | 0.5818 | 0.5779±0.0036 | 0.4907 | 0.4895±0.0001 |
| 7 | 0.5628 | 0.5509±0.0017 | 0.4694 | 0.4683±0.0001 |
| 8 | 0.5458 | 0.5321±0.0047 | 0.4531 | 0.4512±0.0001 |
| 9 | 0.5324 | 0.5156±0.0029 | 0.4403 | 0.4390±0.0002 |
| 11 | 0.5116 | 0.5017±0.0018 | 0.4215 | 0.4202±0.0001 |

Here $P^C_{2d}$ and $P^C_{3d}$ represent the maximum success probabilities of $2^{(d)} \to 1$ and $3^{(d)} \to 1$ classical RACs.

# References


[1] F. Mezzadri, Notices of the American Mathematical Society **54**, 592 (2007).

[2] S. Designolle, P. Skrzypczyk, F. Fröwis, N. Brunner, Phys. Rev. Lett. **122**, 050402 (2019).
